# Supplementary material for: Annotation Free Semantic Segmentation with Vision Foundation Models
Source: arXiv:2403.09307 source file (2024-09-13)
Supplement: Supplementary file 1 [file ablation_all.tex]

\begin{tabular}{l|l|l|l|l|l|l|l|l|l|l}
    \toprule
     \multirow{2}[1]{*}{Method}  &
 \multirow{2}[1]{*}{Training }& \multirow{2}[1]{*}{Annotation }& \multicolumn{7}{c}{mIoU} 
    \\
& &&PV-21&PV-20& PC-59 &CO80 &CS-171&City&ADE&AVG.
  \\
      \midrule
     TCL~\cite{cha2023learning}&CC-15M &Image Level&55.0&83.2 & 33.9& 31.6 & 22.4&24.0&17.1&38.17
\\
   \midrule                       
                                    \multicolumn{1}{c}{\textbf{\ours Training-Free}}
                                    \\
                                    \midrule
                                    Stage.1.1&- &-&42.92& 25.37&22.03&32.97 &16.96&9.50&10.45&22.88
                                    \\
                                    Stage.1.1 - semi&- &Image Level&50.86& 63.82&39.33&47.77 &29.03&10.76&\textbf{22.86}&37.77
                                    \\
                                    Stage.1.2 &- &-&53.36& 36.68&24.25&29.15 &16.82&14.86&12.30&26.77
                                    \\
                                    \midrule
                                    \multicolumn{1}{c}{\textbf{\ours Training-Based}}
                                    \\
                                    \midrule
                Stage 1.1 & COCO-Stuff&-  &  65.83&85.41&41.34&57.56 &28.02&22.15&15.40&45.10
                \\
                Stage 1.1 - finetuned & Target Dataset&-  &  63.22& 86.21&41.92& $57.56^{*}$ & $28.02^{*}$ &25.59&21.54&45.86
                \\
                Stage 1.2 & COCO-Stuff&-  &  63.71& 81.10&38.85&50.86 &26.08&\textbf{30.21}&14.11&43.56
                \\
                Stage 1.2 - finetuned & Target Dataset&-  &  63.09& 82.13&35.92& $50.86^{*}$ & $26.08^{*}$ &28.89&17.77&43.53
                \\
                Stage 1.1 + 1.2 & COCO-Stuff&-  &  67.73&85.65&\textbf{42.72}&\textbf{57.63}&\textbf{29.88}&28.37&16.25&46.89
                \\
                Stage 1.1 + 1.2 - finetuned & Target Dataset&-  &  \textbf{68.87}& \textbf{86.92}&42.49& $57.63^{*}$ & $\textbf{29.88}^{*}$ &26.25&\textbf{21.57}&\textbf{47.65}
                \\

    \bottomrule
    \end{tabular}
