# Supplementary material for: Annotation Free Semantic Segmentation with Vision Foundation Models
Source: arXiv:2403.09307 source file (2024-09-13)
Supplement: Supplementary file 2 [file arch_ablation.tex]

\begin{tabular}{l|l}
\toprule
\footnotesize
      Architecture & mIoU (CS-171) \\
\midrule
     Linear &27.25\\% \%\\
     MLP & 28.90\\
     Transformer block & 29.88\\
\bottomrule
\end{tabular}
